# Supplementary material for: UniMEL: A Unified Framework for Multimodal Entity Linking with Large Language Models
Source: arXiv:2407.16160 source file (2024-08-21)
Supplement: Supplementary file 1 [file appendix.tex]

\appendix
\appendixpage

%%%%%%%%%%%%%%%%%%%%%%%%%%%%%%%%%%%%%%%%%
\section{Prompt Template}

We provide a running example to explain how our method make augmentation for mentions and entities and how to make muti-choice selection. The prompt example is as follows:
\vspace{-0.5em}

\subsection{Mention augmentation}
\vspace{0.8em}

\noindent\fbox{\parbox{0.98\linewidth}{
\colorbox{mygray}
{
\begin{minipage}{0.95\linewidth}

\vspace{1.0em}
\textbf{Prompt:\\}
\centerline{\includegraphics[width=0.5\linewidth]{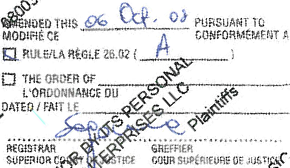}}
\\
The target entity named \textit{Superior Court}.\\
The image describes \textit{The third dated stamp; October 6, 2008. A stamp belonging to the Superior Court with the registrar's signature and mark of acceptance.}\\
Introduce the entity named \textit{Superior Court}. Answer follow the format: "The \textit{Superior Court} refer to..."\\
Only generate an introduction to the target entity, not a description of the image.\\

\textbf{Response:\\}
\textit{Superior Court is a legal organization that operates within a court system, providing a forum for the resolution of disputes and the administration of justice.}

\vspace{1.0em}

\end{minipage}
}
}}

\subsection{Entity augmentation}
\vspace{0.8em}

\noindent\fbox{\parbox{0.98\linewidth}{
\colorbox{mygray}
{
\begin{minipage}{0.95\linewidth}

\vspace{1.0em}
\textbf{Prompt:\\}
Please generate a one-sentence summary for the given entity, including entity name and description.\\
Entity name: \textit{Superior Court (TV series)}\\
Entity description: \textit{Superior Court is a dramatized court show that aired in syndication from 1986 to 1989, and …}\\
\\
Try your best to summarize the main content of the given entity. And generate a short summary in 1 sentence.\\
Summary:\\

\textbf{Response:\\}
\textit{Superior Court was a syndicated court show that aired from 1986 to 1989, featuring fictionalized re-enactments of real court cases, with different judges presiding in each season, including William D. Burns, Jr., Jill Jakes, and Raymond St. Jacques. }

\vspace{1.0em}

\end{minipage}
}
}}

\subsection{Muti-selection}\label{Appendices.3}
\vspace{0.8em}

\noindent\fbox{\parbox{0.98\linewidth}{
\colorbox{mygray}
{
\begin{minipage}{0.95\linewidth}

\vspace{1.0em}
\textbf{Prompt:\\}
You are an expert in knowledge graph, and matching at top k specifically. Your task is to create matches between mention and entity tables to select the best-matched entity to match the given mention.\\

\#\#\# Mention\\
Name: \textit{Superior Court}\\
Context: \textit{The third dated stamp; October 6, 2008. A stamp belonging to the Superior Court with the registrar's signature and mark of acceptance.}\\
Category: \textit{Organization}\\
Description: \textit{Superior Court is a legal organization that operates within a court system, providing a forum for the resolution of disputes and the administration of justice.}\\
\\
\#\#\# Entity table\\
0. : Superior Court (TV series): Superior Court was a syndicated court show that …\\
1. entity1\\
2. entity2\\
3. entity3\\
4. entity4\\
\\
Just give the most matched entity and do not give me any other information.\\
Output a json following the format:\\
\textasciigrave\textasciigrave\textasciigrave json
\\
\{\{\\
\hspace*{0.5cm} "id": "",\\
\hspace*{0.5cm} "name": ""\\
\}\}\\
\textasciigrave\textasciigrave\textasciigrave\\
\\
\textbf{Response:}\\
\textasciigrave\textasciigrave\textasciigrave json
\\
\{\{\\
\hspace*{0.5cm} "id": "0",\\
\hspace*{0.5cm} "name": "Superior Court (TV series)"\\
\}\}\\
\textasciigrave\textasciigrave\textasciigrave\\
\textbf{Ground Truth}: \textcolor{red}{0}

\vspace{1.0em}

\end{minipage}
}
}}

%%%%%%%%%%%%%%%%%%%%%%%%%%%%%%%%%%%%%%%%%
